# Supplementary material for: Evaluating uncertainties in electrochemical impedance spectra of solid oxide fuel cells
Source: arXiv:2101.08049 source file (2021-05-05)
Supplement: Supplementary file 1 [file appendix.tex]

% !TEX root = main.tex

\appendix
